# Supplementary material for: Approach for composition measurement of cosmic rays using the muon-to-electron ratio observed by LHAASO-KM2A
Source: arXiv:2407.13298 source file (2024-07-18)
Supplement: Supplementary file 1 [file appendix.tex]

\appendix
    % \subsection{Energy Binning}
    %     The expected all-particle knee is around $3\si{PeV}$.
    %     On the other hand, the knee stands for the change of the spectrum shape,
    %     which requires wider energy coverage to observe the transition.
    %     Therefore, the energy ranges $10^{5.3-7.3}\si{GeV}$, with a step size of
    %     0.2dex.
    %     The bin width depends on several factors: event statistic, energy resolution
    %     and the change of the primary spectrum.
    %     In addition, Fig \ref{fig:E_rec} shows the energy reconstruction
    %     is better than $0.2$dex (FWHM) above $1\si{PeV}$.
    %     Therefore, a $0.2$dex binning used in $1-10\si{PeV}$ is reasonable.
    % \subsection{Interaction Model}
    %     Composition studies from the ground
    %     are always subject to the uncertainties from hadronic interaction models.
    %     The generally employed approach to
    %     report the uncertainties introduced by hadronic interaction
    %     models is to bracket the difference of the fitting results with different interaction
    %     models. The baseline model is QGSJetII.04.
    %     The alternative model for comparison is Sibyll2.3d.
    %     Both models are post-LHC models,
    %     i.e., tuned to be more compatible with LHC measurements.
    %     The results are shown in Fig \ref{fig:hadronic}.
    %     The estimated uncertainties :
    %     1. the difference between the two hadronic models
    %     are roughly $20\%$ except for Fe.
    %     2. Fe spectrum differs by around $100\%$ for the two models.
\section{Number of secondary particles}
    The number of secondary particles are converted from the photoelectrons
    measured in all detectors (EDs or MDs).
\section{Fitting}
    The normalization factors of five mass groups are free parameters.
    Markov Chain Monte Carlo (MCMC) is used to maximize the likelihood
    of reproducing the observed data. The posterior distributions of the five
    parameters for $E_{\mathrm{rec}}$ from 2.5-4PeV is shown in Fig \ref{fig:corner},
    where the values represent the relative normalization factor with respect
    to the input spectrum,
    i.e. H3a model in this case. An example of the fitted $NuM4/NpE3$ spectrum is
    shown in Fig \ref{fig:fitted_spectrum}. 
    The statistical uncertainties are determined by the $16\%$ and $84\%$ quantiles
    \footnote{$1\sigma$ range for a Gaussian.} in the posteriors.
    % \falta{One caveat for the fitting is that not all fittings converge after XXX steps,
    % where the converge criterion is the chain length is 50 times longer than
    % the auto-correlation time.}

    In other words, the $NuM4/NpE3$ distribution of five mass groups are adjusted vertically
    in every reconstructed energy bin to get the nucleus flux. Figure \falta{XX}
    shows the fit results in 1.3-2.0PeV. The solid line is KM2A data. The dashed line
    is the summation of five mass groups with the best fit normalization factors,
    which shows good agreement with the data.

    On the other hand, \falta{we note that the results are still temporary.}
    A serious analysis
    requires an iterative fitting, which updates the input spectrum
    according to previous output every time
    until the output spectrum does not change. Therefore, the dependence of the fitting
     on the input spectrum is eliminated by the iteration of fitting.

\subsection{Approximate the primary composition with 5 mass groups}
    Decomposing the primary cosmic ray into five mass groups
    neglects the contributions from other nuclei.
    Though the contributions from nuclei besides the five leading
    mass groups are probably small, such approximation
    will introduce systematic uncertainties in the primary composition.
